# Supplementary material for: Strange metal and superconductor in the two-dimensional Yukawa-Sachdev-Ye-Kitaev model
Source: arXiv:2406.07608 source file (2024-11-15)
Supplement: Supplementary file 1 [file supp3.pdf]

# SUPPLEMENT TO

## Strange metal and superconductor in the two-dimensional Yukawa-SYK model

Chenyuan Li,<sup>1</sup> Davide Valentinis,<sup>2,3</sup> Aavishkar A. Patel,<sup>4</sup>  
Haoyu Guo,<sup>5</sup> Jörg Schmalian,<sup>2,3</sup> Subir Sachdev,<sup>1</sup> and Ilya Esterlis<sup>6</sup>

<sup>1</sup>*Department of Physics, Harvard University, Cambridge MA 02138, USA*

<sup>2</sup>*Institut für Quantenmaterialien und Technologien,  
Karlsruher Institut für Technologie, 76131 Karlsruhe, Germany*

<sup>3</sup>*Institut für Theorie der Kondensierten Materie,  
Karlsruher Institut für Technologie, 76131 Karlsruhe, Germany*

<sup>4</sup>*Center for Computational Quantum Physics,  
Flatiron Institute, New York, New York, 10010, USA*

<sup>5</sup>*Laboratory of Atomic and Solid State Physics, Cornell University,  
142 Sciences Drive, Ithaca NY 14853-2501, USA*

<sup>6</sup>*Department of Physics, University of Wisconsin-Madison, Madison, Wisconsin 53706, USA*

(Dated: June 19, 2024)

The plan of the supplement is as follows. We introduce our model, its averaged effective action, and the setup of the large- $N$  expansion in Section [SI](#). This involves a path integral over a  $G - \Sigma$  action in which the fields are bilocal in spacetime. A full numerical solution of the large  $N$  equations for the complete Fermi surface is obtained in Section [SII](#) for complex couplings and [SIII](#) for real couplings. We present the normal state and superconducting solutions and find results which are in agreement with the previous analysis. We then discuss transport properties in Section [SIV](#), and Homes' Law in Section [SV](#).

## SI. THE 2d-YSYK MODEL AND ITS SADDLE-POINT EQUATIONS

We endow the fermions and bosons with an additional flavor index  $i, j, \ell$ , and the fermions with a spin index  $\sigma$ , and work the following lattice action in imaginary time

$$\begin{aligned}
S = & \int d\tau d^2x \sum_{i=1}^N \sum_{\sigma=\pm 1} \psi_{i\sigma}^\dagger(\tau, x) [\partial_\tau + \varepsilon_k] \psi_{i\sigma}(\tau, x) + \frac{1}{2} \int d\tau d^2x \sum_{i=1}^N \phi_i(\tau, x) [-\partial_\tau^2 + \omega_q^2] \phi_i(\tau, x) \\
& + \int d^2\tau dx \sum_{i,j}^N \sum_{\sigma=\pm 1} \frac{v_{ij}(x)}{\sqrt{N}} \psi_{i\sigma}^\dagger(\tau, x) \psi_{j\sigma}(\tau, x) \\
& + \int d\tau d^2x \sum_{i,j,\ell=1}^N \sum_{\sigma=\pm 1} \frac{g'_{ij\ell}(x)}{N} \psi_{i\sigma}^\dagger(\tau, x) \psi_{j\sigma}(\tau, x) \phi_\ell(\tau, x), \tag{S1}
\end{aligned}$$

with the following choice of lattice dispersion

$$\epsilon_k = -2t(\cos k_x + \cos k_y) - \mu, \tag{S2a}$$

$$\omega_q^2 = m_b^2 + 2J(2 - \cos q_x - \cos q_y). \tag{S2b}$$

Here  $t$  is the fermion hopping,  $\mu$  is the chemical potential,  $m_b$  is the bare boson mass and the stiffness  $J$  determines the boson dispersion. The Yukawa couplings  $g'_{ij\ell}$  are complex-valued random variables that obey  $g'_{ij\ell}(x) = g_{1,ij\ell}(x) + i g_{2,ij\ell}(x) = g'_{ji\ell}(x)$ . The real part  $g_{1,ij\ell}(x)$  and the imaginary part  $g_{2,ij\ell}(x)$  have zero mean and the variances are [\[1\]](#)

$$\begin{aligned}
\overline{g_{1,ij\ell}(x) g_{1,i'j'\ell'}(x')} &= \left(1 - \frac{\alpha}{2}\right) g'^2 \delta_{\ell,\ell'} (\delta_{ii'} \delta_{jj'} + \delta_{ij'} \delta_{ji'}) \delta(x - x'), \\
\overline{g_{2,ij\ell}(x) g_{2,i'j'\ell'}(x')} &= \frac{\alpha}{2} g'^2 \delta_{\ell,\ell'} (\delta_{ii'} \delta_{jj'} - \delta_{ij'} \delta_{ji'}) \delta(x - x'), \\
\overline{g_{1,ij\ell}(x') g_{2,i'j'\ell'}(x')} &= 0. \tag{S3}
\end{aligned}$$

In the  $\alpha = 1$  limit, [\(S3\)](#) reduces to  $\langle g'_{ij\ell}(x) g'_{i'j'\ell'}(x')^* \rangle = g'^2 \delta(x - x') \delta_{ii'} \delta_{jj'} \delta_{\ell\ell'}$  and no superconductivity occurs [\[1\]](#). For  $\alpha = 0$ , however, the coupling constants are all real valued, which

preserves time-reversal symmetry for each realization of the random couplings and thus gives rise to superconductivity. The spatially random potential satisfies

$$\overline{v_{ij}(x)} = 0, \quad \overline{v_{ij}^*(x)v_{i'j'}(x')} = v^2 \delta(x - x') \delta_{ii'} \delta_{jj'}, \quad (\text{S4})$$

After a disorder average via the replica trick, we obtain

$$\begin{aligned} \frac{S}{N} = & -\text{Tr} \log(\hat{G}_0^{-1} - \hat{\Sigma}) + \frac{1}{2} \text{Tr} \log(D_0^{-1} - \Pi) \\ & - \int d\tau d^2x \int d\tau' d^2x' \left( 2\Sigma(\tau', x'; \tau, x) G(\tau, x; \tau', x') - \frac{1}{2} \Pi(\tau', x'; \tau, x) D(\tau, x; \tau', x') \right) \\ & - \int d\tau d^2x \int d\tau' d^2x' \left( \Phi^\dagger(\tau', x'; \tau, x) F(\tau, x; \tau', x') + \Phi(\tau', x'; \tau, x) F^\dagger(\tau, x; \tau', x') \right) \\ & + v^2 \int d\tau d^2x \int d\tau' d^2x' (G(\tau, x; \tau', x') G(\tau', x'; \tau, x) - (1 - \alpha) F^\dagger(\tau, x; \tau', x') F(\tau', x'; \tau, x)) \delta(x - x') \\ & + g'^2 \int d\tau d^2x \int d\tau' d^2x' G(\tau, x; \tau', x') G(\tau', x'; \tau, x) D(\tau, x; \tau', x') \delta(x - x') \\ & - g'^2 (1 - \alpha) \int d\tau d^2x \int d\tau' d^2x' F^\dagger(\tau, x; \tau', x') F(\tau', x'; \tau, x) D(\tau, x; \tau', x') \delta(x - x') \\ & - \int d\tau d^2x \frac{i\lambda(\tau, x)}{2} \left( \sum_{i=1}^N \phi_i(\tau, x) \phi_i(\tau, x) - N/\gamma \right). \end{aligned} \quad (\text{S5})$$

Here  $\hat{G}_0^{-1}$  and  $\hat{\Sigma}$  are matrices in Nambu space. We have introduced the time-bilocal fields  $G$ ,  $F$ ,  $D$ , which are normal and anomalous fermionic Green's functions, as well as bosonic Green's functions. The corresponding self-energies, given by  $\Sigma$ ,  $\Phi$  and  $\Pi$ , are employed as Lagrange multipliers. To tune the system to criticality, we have found it most convenient to first impose a fixed length constraint [2]:

$$\sum_q \sum_{i=1}^N \phi_{iq}(\tau) \phi_{i,-q}(\tau) = N/\gamma, \quad (\text{S6})$$

which is implemented by the Lagrange multiplier  $\lambda$  Eq.(S6) and implicitly determines  $m_b^2$ , and use  $\gamma$  as tuning parameter to access the QCP. In the main text we present the phase diagram in terms of the  $T = 0$  value of the renormalized boson mass  $M^2 = m_b^2 - \Pi(\omega = 0, T = 0)$ .

Integrating out  $\psi$  and  $\phi$  yields this  $G$ - $\Sigma$  action (S5). In the limit of a large number of flavors,

the SYK-type saddle-point equations are given by

$$\hat{G}(i\omega) = \int \frac{d^2k}{(2\pi)^2} \left( i\omega\sigma_0 + \mu\sigma_3 - \varepsilon_k\sigma_3 - \hat{\Sigma}(i\omega) \right)^{-1}, \quad (\text{S7a})$$

$$D(i\nu) = \int \frac{d^2q}{(2\pi)^2} \frac{1}{\nu^2 + \omega_q^2 + m_b^2 - \Pi(i\nu)}, \quad (\text{S7b})$$

$$\Sigma(\tau) = g'^2 G(\tau) D(\tau) + v^2 G(\tau), \quad (\text{S7c})$$

$$\Phi(\tau) = -(1 - \alpha)(g'^2 F(\tau) D(\tau) + v^2 F(\tau)), \quad (\text{S7d})$$

$$\Pi(\tau) = -2g'^2 (G(\tau)G(-\tau) - (1 - \alpha)F(\tau)F^\dagger(-\tau)), \quad (\text{S7e})$$

$$\frac{1}{\gamma} = T \sum_\nu \int \frac{d^2q}{(2\pi)^2} \frac{1}{\nu^2 + \omega_q^2 + m_b^2 - \Pi(i\nu)}. \quad (\text{S7f})$$

These equations are indicated schematically in Figure 1 for  $v = 0$ . Different from the translationally invariant model, the self-energies are momentum independent as a result of the extra  $\delta$ -function in (S5). In section SII and SIII we will present numerical solutions of these equations.

## SII. NUMERICAL SOLUTIONS TO THE COMPLEX 2d-YSYK MODEL

We first solve the saddle-point equations in the normal state and consider complex-valued  $g'_{ij\ell}$  extracted from the Gaussian unitary ensemble ( $\alpha = 1$ )[1, 3]. In this limit, the anomalous terms disappear and saddle point equations (S7a)-(S7e) are simplified as

$$\Sigma(i\omega_n) = g'^2 T \sum_m G(i\omega_n - i\nu_m) D(i\nu_m) + v^2 G(i\omega_n), \quad (\text{S8a})$$

$$\Pi(i\nu_n) = -2g'^2 T \sum_m G(i\nu_n + i\omega_m) G(i\omega_m), \quad (\text{S8b})$$

$$G(i\omega_n) = \int \frac{d^2k}{(2\pi)^2} \frac{1}{i\omega_n - \varepsilon_k + \mu - \Sigma(i\omega_n)}, \quad (\text{S8c})$$

$$D(i\nu_n) = \int \frac{d^2q}{(2\pi)^2} \frac{1}{\nu_n^2 + \omega_q^2 + m_b^2 - \Pi(i\nu_n)}. \quad (\text{S8d})$$

For the lattice dispersion (S2), the momentum integrations for the local Green's functions can be worked out analytically, giving rise to the local Green's function

$$G_{\text{loc}}(z) = \frac{1}{4t} \mathcal{G} \left( \frac{z + \mu - \Sigma(z)}{4t} \right). \quad (\text{S9})$$

Here we define

$$\mathcal{G}(z) \equiv \frac{2}{\pi z} K(1/z^2), \quad (\text{S10})$$

with  $K$  the complete elliptic integral of the first kind. Similarly, for the bosons we obtain

$$D_{\text{loc}}(z) = \frac{1}{4J} \mathcal{G} \left( \frac{z^2 - m_b^2 - 4J - \Pi(z)}{4J} \right), \quad (\text{S11})$$

where  $m_b^2$  is obtained by solving the above equations with the constraint (S7f)

$$D_{\text{loc}}(\tau = 0) = -\frac{1}{\gamma}. \quad (\text{S12})$$

The value of  $m_b^2$  thus obtained will be plugged into the equations expressed on the real-axis below. Notice that because we have taken care of the momentum integration analytically, we work directly in the thermodynamic limit. The integral equations above are most efficiently solved via fast Fourier transform (FFT). In our calculations, we have used the imaginary time-Matsubara frequency FFT approach described in Ref. [4].

The real-axis version of (S8) originates from the analytic continuation  $i\omega_n \rightarrow \omega + i0^+$  of imaginary propagators. To proceed, we introduce the following spectral functions

$$A(\omega) = -\frac{1}{\pi} \text{Im} G^R(\omega), \quad (\text{S13a})$$

$$B(\omega) = -\frac{1}{\pi} \text{Im} D^R(\omega), \quad (\text{S13b})$$

where  $G^R(\omega) = G(i\omega_n)|_{i\omega_n \rightarrow \omega + i0^+}$  and  $D^R(\omega) = D(i\nu_n)|_{i\nu_n \rightarrow \omega + i0^+}$  are the retarded Green's functions. From the spectral representation, we derive the following retarded self energies

$$\Sigma_R(\omega) = g'^2 \int_{\omega'} \left[ \tilde{A}(\omega') D_R(\omega - \omega') - \tilde{B}(\omega') G_R(\omega + \omega') \right] + v^2 G_R(\omega), \quad (\text{S14a})$$

$$\Pi_R(\omega) = g'^2 \int_{\omega'} \tilde{A}(\omega') ([G_R(\omega' - \omega)]^* + G_R(\omega + \omega')), \quad (\text{S14b})$$

Here we define  $\tilde{A}(\omega) \equiv A(\omega)n_F(\omega)$  and  $\tilde{B}(\omega) \equiv B(\omega)n_B(\omega)$ . This approach is similar to that developed in [5].

Numerical results in this section are presented for the fermion chemical potential  $\mu = -0.5t$ , boson stiffness  $J = t^2$ , and impurity potential  $v = 0$ .

### A. Boson properties

The temperature-dependent renormalized boson mass is  $M^2(T) = m_b^2 - \Pi(\omega = 0, T)$  [2]. At the QCP,  $M^2(T) \sim T$  at low temperatures (up to logarithms), as is seen in the left panel of Figure S1. When we simply write  $M^2$ , we refer to the  $T = 0$  value  $M^2 = M^2(T = 0)$ . The retarded boson self-energy shown in Figure S1 obeys  $-\text{Im}\Pi_R \sim \omega$ , the expected Landau damping form, corresponding to dynamical exponent  $z = 2$ . The low-frequency behavior is essentially independent of the distance to the QCP.

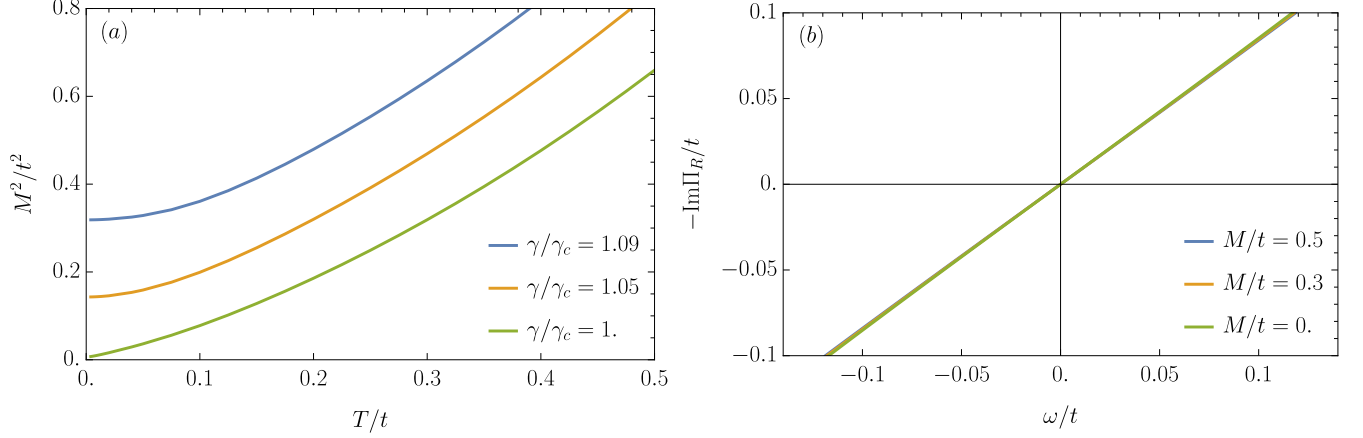

FIG. S1: (a) Renormalized boson mass as a function of  $T$  at  $g'/t^{3/2} = 2$  for  $\gamma \geq \gamma_c$ , where  $\gamma_c$  is the QCP and  $\gamma > \gamma_c$  corresponds the Fermi-liquid side of the phase diagram. (b) Imaginary part of the bosonic self-energy as a function of  $\omega/t$  at  $T/t = 0.004$  for different values of  $T = 0$  boson mass.

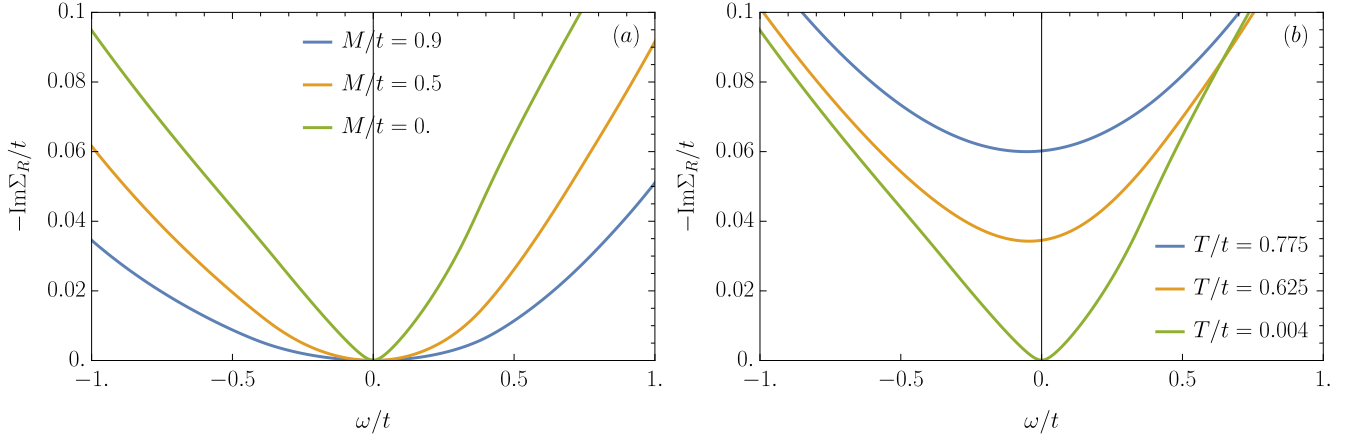

FIG. S2: (a) Imaginary part of the fermionic self-energy as a function of  $\omega/t$  at  $T/t = 0.004$ ,  $g'/t^{3/2} = 2$  for different values of the boson mass. (b) Same as (a) but at the QCP for different temperatures.

## B. Fermion properties

Figure S2 shows the imaginary part of the fermionic self-energy, which has the expected forms: a marginal Fermi liquid at the QCP,  $-\text{Im}\Sigma_R \sim |\omega|$ , and  $-\text{Im}\Sigma_R \sim \omega^2$  in the FL regime. The mass enhancement extracted from the fermion self-energy is shown in Fig. S3.

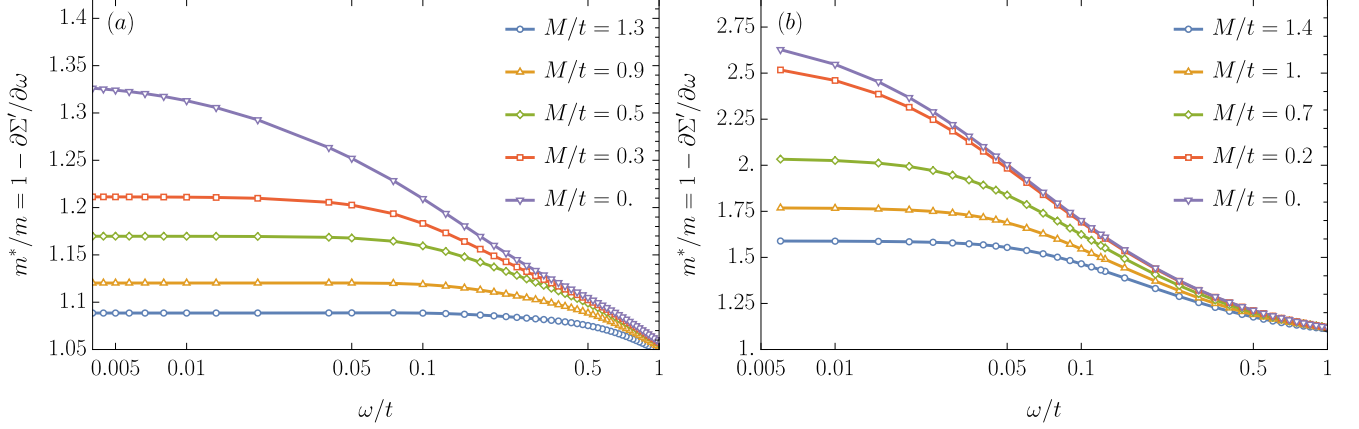

FIG. S3: Enhancement of the effective mass as a function of  $T/t$  for different values of boson mass. (a)  $g'/t^{3/2} = 2$  (weak coupling) (b)  $g'/t^{3/2} = 5$  (strong coupling).

### SI. NUMERICAL SOLUTIONS TO THE REAL 2d-YSYK MODEL

#### A. Linearized gap equations and $T_c$

Now we turn to real-valued  $g'_{ij\ell}$  extracted from the Gaussian orthogonal ensemble [1, 3], and start from the linearized gap equations

$$\Phi(i\omega_n) = g'^2(1 - \alpha)T \sum_m D(i\omega_n - i\omega_m)X(i\omega_m)\Phi(i\omega_m) + v^2(1 - \alpha)X(i\omega_n)\Phi(i\omega_n). \quad (\text{S15})$$

Here  $X(i\omega_m)$  is determined by normal state solutions

$$X(i\omega_m) = \frac{G^N(i\omega_m) - G^N(-i\omega_m)}{2i\omega_m - \Sigma(i\omega_m) + \Sigma(-i\omega_m)}, \quad G^N(i\omega_m) = \frac{1}{4t} \mathcal{G} \left( \frac{i\omega_m + \mu - \Sigma(i\omega_m)}{4t} \right). \quad (\text{S16})$$

After introducing

$$\tilde{\Phi}(i\omega_n) \equiv \Phi(i\omega_n)[1 - v^2(1 - \alpha)X(i\omega_n)], \quad (\text{S17})$$

Eq. S15 reduces to

$$\tilde{\Phi}(i\omega_n) = g'^2(1 - \alpha)T \sum_m D(i\omega_n - i\omega_m) \frac{1}{1/X(i\omega_m) - v^2(1 - \alpha)} \tilde{\Phi}(i\omega_m). \quad (\text{S18})$$

Therefore, the superconducting transition temperature  $T_c$  can be determined by imposing that the matrix

$$K_{nm} = g'^2(1 - \alpha)TD(i\omega_n - i\omega_m) \frac{1}{1/X(i\omega_m) - v^2(1 - \alpha)}, \quad (\text{S19})$$

has eigenvalue 1. In Fig. S4, we present the superconducting  $T_c$  as a function of tuning parameter

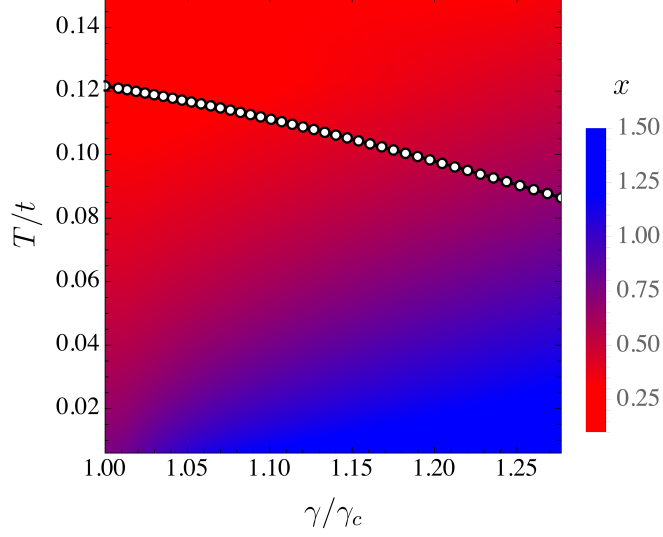

FIG. S4: Phase diagram as  $x(\gamma, T/t)$ . Up to logarithmic corrections, we expect  $x = 1$  (blue) in the quantum critical fan and  $x = 2$  in the Fermi liquid regime. White dots indicate  $T_c$ . The choice of parameters:  $\mu = -0.5t$ ,  $J = t^2$ ,  $g' = 5t^{3/2}$ . Here we set  $\alpha = 0$ ; i.e., purely real couplings.

$\gamma$  in the phase diagram at strong coupling  $g' = 5t^{3/2}$ . The white dots are the superconducting  $T_c$ . The color scale shows the exponent,  $x$ , with which the boson mass approaches its  $T = 0$  value:  $M^2(T) - M^2(T = 0) \sim T^x$ . For  $\gamma > \gamma_c$ , the system behaves as a Fermi liquid with  $x \simeq 2$  at low temperatures, while up to logarithmic corrections, we expect  $x = 1$  at the QCP and within the quantum critical fan. The maximal  $T_c$  occurs just above the critical point. This figure is complementary to Fig. 2 of the main text, which shows the resistivity exponent.

We have also studied the correlation between  $A$  – the slope of the  $T$  linear resistivity – and  $T_c$  when the system is tuned precisely to the QCP at  $\gamma_c$  ( $M = 0$ ). In this case  $T_c$  is tuned by varying the interaction strength  $g'$ . We find an essentially linear relationship, as may be seen in Fig. S5(a). The corresponding tuning parameter  $\gamma_c$  as a function of  $g'$  is shown in Fig. S5(b).

## B. Full solutions to the coupled saddle point equations

Here we present the full solution to the saddle-point equations below the superconducting  $T_c$ . The momentum integrations can also be worked out analytically for the local Green's functions

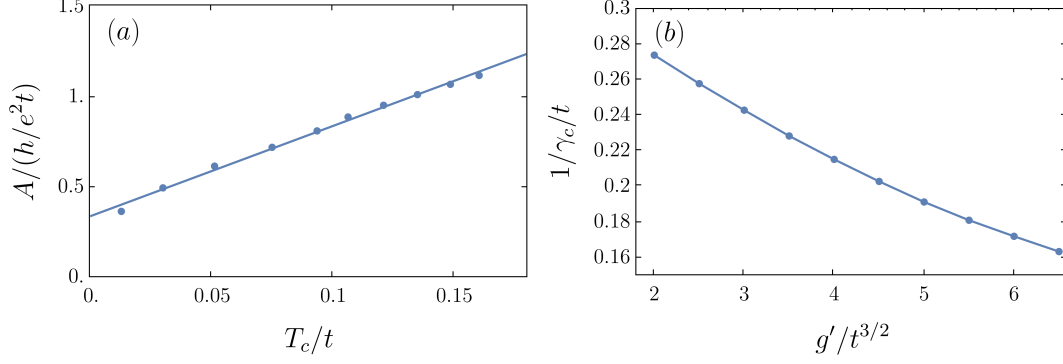

FIG. S5: (a) Relationship between slope  $A$  of the linear in  $T$  resistivity and transition temperature  $T_c$ . Here  $T_c$  is varied by varying  $g'$  while keeping the system at the QCP. (b) The (inverse) value of the tuning parameter  $\gamma$  at the critical point as a function of  $g'$ .

(S7a). Using the lattice dispersion (S2), we have a generalized version of (S9):

$$G_{\text{loc}}(z) = \frac{1}{2} \left( 1 + \frac{zZ(z)}{\sqrt{(zZ(z))^2 - \Phi(z)^2}} \right) \frac{1}{4t} \mathcal{G} \left( \frac{-\chi(z) + \mu + \sqrt{(zZ(z))^2 - \Phi(z)^2}}{4t} \right) + \frac{1}{2} \left( 1 - \frac{zZ(z)}{\sqrt{(zZ(z))^2 - \Phi(z)^2}} \right) \frac{1}{4t} \mathcal{G} \left( \frac{-\chi(z) + \mu - \sqrt{(zZ(z))^2 - \Phi(z)^2}}{4t} \right), \quad (\text{S20a})$$

$$F_{\text{loc}}(z) = \frac{\Phi(z)}{2\sqrt{(zZ(z))^2 - \Phi(z)^2}} \frac{1}{4t} \mathcal{G} \left( \frac{-\chi(z) + \mu + \sqrt{(zZ(z))^2 - \Phi(z)^2}}{4t} \right) - \frac{\Phi(z)}{2\sqrt{(zZ(z))^2 - \Phi(z)^2}} \frac{1}{4t} \mathcal{G} \left( \frac{-\chi(z) + \mu - \sqrt{(zZ(z))^2 - \Phi(z)^2}}{4t} \right). \quad (\text{S20b})$$

Here we define

$$\Sigma(z) + \Sigma(-z) \equiv 2\chi(z), \quad (\text{S21})$$

$$\Sigma(z) - \Sigma(-z) \equiv 2z(1 - Z(z)). \quad (\text{S22})$$

The Green's functions (S20) reduces to (S9) when  $\Phi(z) = 0$ . The analytic continuation  $i\omega_n \rightarrow \omega + i0^+$  of (S20) leads to the retarded Green's functions on the real axis. Following a similar procedure to that shown in SII, we obtain the retarded self energies. The result is most compactly expressed in the real-time domain

$$\Sigma_R(t) = ig'^2(2\pi)^2\theta(t)[\tilde{A}(t)B(t) - \tilde{B}(-t)A(t)], \quad (\text{S23a})$$

$$\Phi_R(t) = -i(1 - \alpha)g'^2(2\pi)^2\theta(t)[\tilde{A}_F(t)B(t) - \tilde{B}(-t)A_F(t)], \quad (\text{S23b})$$

$$\begin{aligned} \Pi_R(t) = i2g'^2(2\pi)^2\theta(t)[\tilde{A}(t)A(-t) - \tilde{A}(-t)A(t), \\ - (1 - \alpha)(\tilde{A}_F(t)A_F(-t) - \tilde{A}_F(-t)A_F(t))]. \end{aligned} \quad (\text{S23c})$$

The self-consistent equations can also be readily solved directly on the real-axis for the retarded functions.

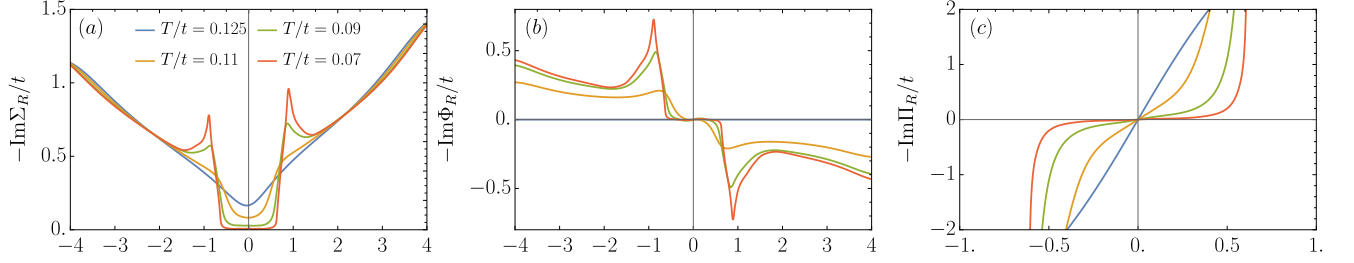

FIG. S6: (a)  $-\text{Im}\Sigma_R$  at QCP ( $\gamma = \gamma_c$ ) for different temperatures. (b)  $-\text{Im}\Phi_R$  at the QCP. (c)  $-\text{Im}\Pi_R$  at QCP.  $-\text{Im}\Pi_R \sim \omega$  in the normal state. The coupling strength is  $g' = 5t^{3/2}$ .

The fermion self-energies and spectral functions are shown in Fig. 4 in the main text. In Fig. S6 we present the normal and anomalous self-energies. In Fig. S7 we report the spectral functions. The figures are all for parameters values  $\mu = -0.5t$ ,  $J = t^2$ ,  $g' = 5t^{3/2}$ , and  $v = 0$ .

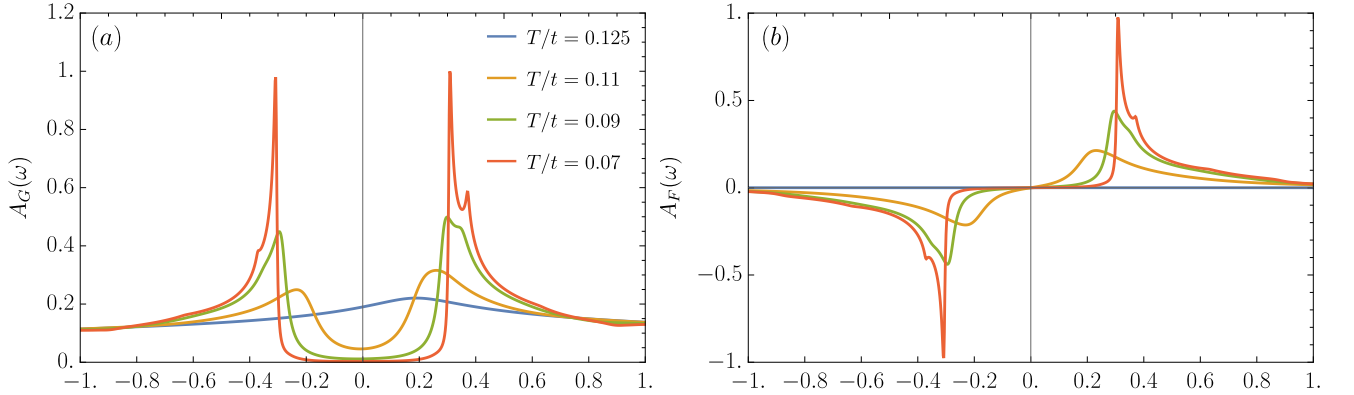

FIG. S7: Spectral functions associated to the normal (a) and anomalous (b) Green's functions. The interaction strength is  $g' = 5t^{3/2}$ .

#### SIV. CONDUCTIVITY AND SUPERFLUID STIFFNESS

The section describes our analysis of the optical conductivity and superfluid stiffness, which may be calculated after the self-consistent Green's functions have been obtained.

### A. Current-current correlator

Consider the current-current correlation function  $\Lambda(\mathbf{q}, \tau) = \langle T_\tau(j_\mu(\mathbf{q}, \tau)j_\nu(-\mathbf{q}, 0)) \rangle$  with

$$\begin{aligned} j_0(\mathbf{q}) &= \sum_{v_{\mathbf{k}}, \sigma} c_{\mathbf{k}, \sigma}^\dagger c_{\mathbf{k}+\mathbf{q}, \sigma} \\ \mathbf{j}(\mathbf{q}) &= \sum_{v_{\mathbf{k}}, \sigma} v_{\mathbf{k}} c_{\mathbf{k}, \sigma}^\dagger c_{\mathbf{k}+\mathbf{q}, \sigma}. \end{aligned} \quad (\text{S24})$$

Here we set the electron charge  $e = 1$ , but will reinstate it in the final results below. At external  $\mathbf{q} = 0$ , the current-current response is just the dressed bubble as seen in Figure 1:

$$\begin{aligned} \Lambda_{\alpha\beta}(i\omega_n) &= -T \sum_{n'} \int_{\mathbf{k}} v_{\mathbf{k}\alpha} v_{\mathbf{k}\beta} \left( G_{\mathbf{k}}(i\omega_{n'}) G_{\mathbf{k}}(i\omega_n + i\omega_{n'}) + F_{\mathbf{k}}^\dagger(i\omega_{n'}) F_{\mathbf{k}}(i\omega_n + i\omega_{n'}) \right) \\ &= -T \sum_{n'} \int d\epsilon \rho_{\text{tr}}^{\alpha\beta}(\epsilon) \left( G(\epsilon, i\omega_{n'}) G(\epsilon, i\omega_n + i\omega_{n'}) + F^\dagger(\epsilon, i\omega_{n'}) F(\epsilon, i\omega_n + i\omega_{n'}) \right). \end{aligned} \quad (\text{S25})$$

In the last step we introduced the “transport” DOS

$$\rho_{\text{tr}}^{\alpha\beta}(\epsilon) = \int_{\mathbf{k}} \frac{\partial \varepsilon_{\mathbf{k}}}{\partial k_\alpha} \frac{\partial \varepsilon_{\mathbf{k}}}{\partial k_\beta} \delta(\epsilon - \varepsilon_{\mathbf{k}}) \quad (\text{S26})$$

and used the fact that the normal and anomalous self energies are momentum independent. For the given dispersion (S2), this quantity is analytically computable

$$\rho_{\text{tr}}(\epsilon) = \frac{2t}{\pi^2} \left[ E(1 - \epsilon^2/16t^2) - \frac{\epsilon^2}{16t^2} K(1 - \epsilon^2/16t^2) \right], \quad (\text{S27})$$

where  $E$  is the complete elliptic integral of the second kind. In the normal state, the analytic continuation for the retarded ( $R$ ) function is

$$\Lambda_R(\omega) = \int d\epsilon \rho_{\text{tr}}(\epsilon) \int d\omega' n_F(\omega') A(\epsilon, \omega') \{ G_R(\epsilon, \omega + \omega') + [G_R(\epsilon, \omega' - \omega)]^* \}, \quad (\text{S28})$$

where  $n_F$  is the Fermi function. The final expression is efficiently evaluated via FFTs by rewriting the convolution in real-time:

$$\Lambda_R(t) = \int d\epsilon \rho_{\text{tr}}(\epsilon) \times 2\pi \{ [\tilde{A}(\epsilon, t)]^* G_R(\epsilon, t) + \tilde{A}(\epsilon, t) [G_R(\epsilon, t)]^* \}. \quad (\text{S29})$$

### B. Conductivity

The conductivity is related to  $\Lambda_R$  according to

$$\sigma(\omega) = -\frac{\langle -K \rangle / d - \Lambda_R(\omega)}{i(\omega + i\delta)}, \quad (\text{S30})$$

where  $\langle -K \rangle$  is the (negative of) the average kinetic energy per site and  $d$  is the spatial dimension (for us  $d = 2$ ). Explicitly

$$K = -t \sum_{\langle ij \rangle, \sigma} (c_{i\sigma}^\dagger c_{j\sigma} + \text{h.c.}). \quad (\text{S31})$$

We may write

$$\sigma(\omega) = D\delta(\omega) + \sigma_{\text{reg}}(\omega) \quad (\text{S32})$$

where the Drude weight is

$$D = \pi[\langle -K/2 \rangle - \Lambda'_R(\omega \rightarrow 0)] \quad (\text{S33})$$

and

$$\sigma_{\text{reg}}(\omega) = \frac{\Lambda''_R(\omega)}{\omega} - i \frac{\Lambda'_R(\omega) - \langle -K/2 \rangle}{\omega}. \quad (\text{S34})$$

In a disordered system, the  $\delta$ -function contribution vanishes (there is a finite dc resistance), from which we find

$$D = 0 \Rightarrow \langle -K/2 \rangle = \Lambda'_R(\omega \rightarrow 0) \quad (\text{S35})$$

and we may also write

$$\sigma(\omega) = \frac{\Lambda''_R(\omega)}{\omega} - i \frac{\Lambda'_R(\omega) - \Lambda'_R(\omega \rightarrow 0)}{\omega} \quad (\text{disordered system}). \quad (\text{S36})$$

This form is useful since it does not require computing independently  $\langle K \rangle$  (although explicitly comparing the left- and right-hand sides of Eq. (S35) is a useful consistency check). Another useful result that follows from Kramers-Kronig is the sum rule

$$\int_{-\infty}^{\infty} d\omega \sigma(\omega) = \pi \langle -K/2 \rangle. \quad (\text{S37})$$

Finally, note the dc limit for the conductivity can also be taken explicitly:

$$\sigma_{\text{dc}} = \lim_{\omega \rightarrow 0} \frac{\Lambda''_R(\omega)}{\omega} = \pi \int d\epsilon \rho_{\text{tr}}(\epsilon) \int d\omega' \left( -\frac{\partial n_F}{\partial \omega'} \right) [A(\epsilon, \omega')]^2. \quad (\text{S38})$$

As described in the main text, we have parametrized the conductivity in the form [6]

$$\sigma(\omega) = i \frac{e^2 K/2}{\omega \frac{m^*(\omega)}{m} + \frac{i}{\tau_{\text{tr}}(\omega)}}, \quad (\text{S39})$$

and so determine a frequency dependent effective mass enhancement  $m^*(\omega)/m$  and transport scattering time  $\tau_{\text{tr}}(\omega)$ . We show the results in Figs. S8. We also show results for the absolute value and phase of the complex conductivity in Fig. S8 (e-f), with results which are very similar to the corresponding results of Michon *et al.* [6].

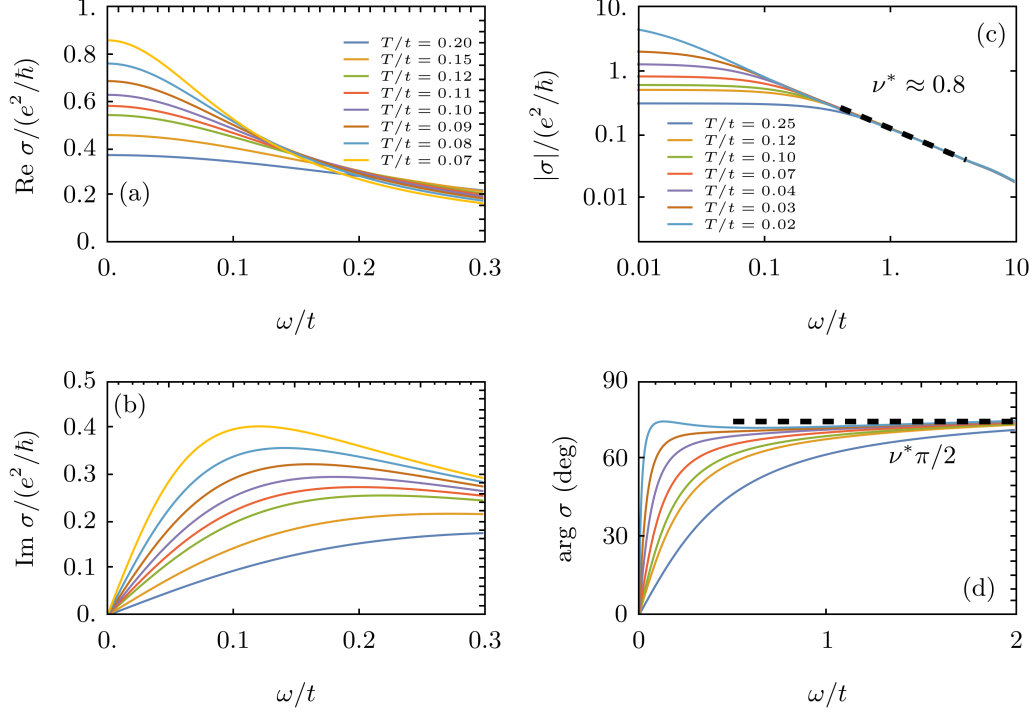

FIG. S8: Optical conductivity at larger coupling  $g' = 5t^{3/2}$  and  $v = 0$ . (a,b) Normal state optical conductivity at the quantum critical coupling for various temperatures indicated in Panel (a). (c,d) Modulus and phase of  $\sigma(\omega)$  with temperatures indicated in Panel (c).

Another way to extract the transport scattering time is motivated from the Drude formula:

$$\sigma'_{\text{Drude}}(\omega) = \sigma_{\text{dc}} \frac{1}{1 + (\omega \tilde{\tau}_{\text{tr}})^2} \quad (\text{S40})$$

This motivates the identification more generally:

$$\frac{\sigma_{\text{dc}}}{\sigma'(\omega)} - 1 = (\omega \tilde{\tau}_{\text{tr}})^2 + \dots \quad (\text{S41})$$

where  $\dots$  denote terms higher order in  $\omega$ . From the fits we may extract  $\tilde{\tau}_{\text{tr}}$  from Eq. (S41): Writing  $\tilde{\tau}_{\text{tr}}^{-1} = \alpha T$  we see that (1)  $\alpha$  is a function of  $T$  for  $T \lesssim 0.1t$  and (2) for  $T \gtrsim 0.1t$  we have  $\alpha \simeq 0.4$ .

### C. Superfluid stiffness

The coefficient  $D$  of the delta function, the Drude weight, can be obtained by extrapolating  $i\omega_n \rightarrow 0$  [7]. If there is a gap,  $D = \rho_s$ , and the superfluid stiffness is

$$\frac{\rho_s}{\pi e^2} = \langle -K \rangle / 2 - \Lambda(i\omega_n = 0), \quad (d = 2). \quad (\text{S42})$$

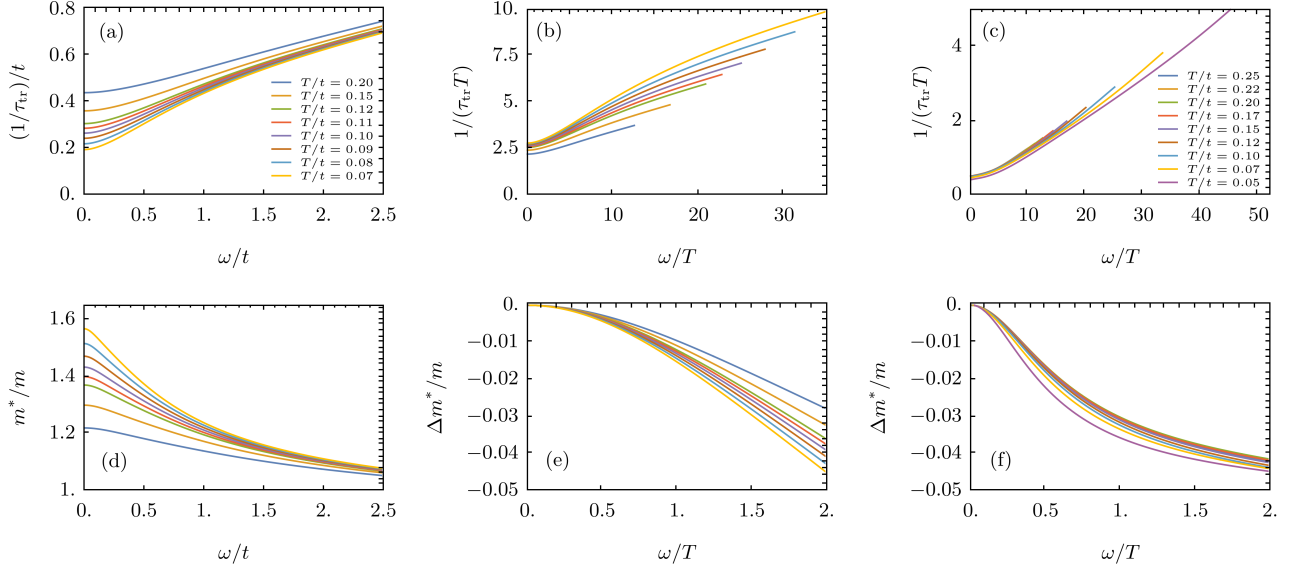

FIG. S9: (a,d) Transport scattering rate  $1/\tau_{\text{tr}}$  and effective mass  $m^*$  obtained from  $\sigma$  using (3) at larger coupling  $g' = 5t^{3/2}$ . (b) A scaling plot with  $1/\tau_{\text{tr}}$  and  $\omega$  scaled by  $T$  at  $g' = 5t^{3/2}$ . (c) Same as (b) at  $g' = 2t^{3/2}$ . (e) A scaling plotting showing  $\Delta m^*/m = m^*(\omega)/m - m^*(0)/m$  as a function of  $\omega/T$  at  $g' = 5t^{3/2}$ . (f) Same as (e) at  $g' = 2t^{3/2}$ .

The two weighted densities of states  $\rho_{\text{tr}}(\epsilon) \equiv \frac{1}{N} \sum_k v_k^2 \delta(\epsilon - \epsilon_k)$  and  $\rho_0(\epsilon) \equiv \frac{1}{N} \sum_k \delta(\epsilon - \epsilon_k)$  are closely related with each other

$$\frac{d\rho_{\text{tr}}(\epsilon)}{d\epsilon} = -\frac{\epsilon}{2}\rho_0(\epsilon). \quad (\text{S43})$$

Therefore, we can rewrite the average kinetic energy per site as

$$\begin{aligned} \langle K \rangle &= \frac{1}{\beta} \sum_{\omega_n} \frac{1}{N} \sum_k \epsilon_k G(k, i\omega_n) e^{i\omega_n 0^+} = \frac{1}{\beta} \sum_{\omega_n} \int d\epsilon \rho_0(\epsilon) \epsilon G(\epsilon, i\omega_n) e^{i\omega_n 0^+} \\ &= -\frac{2}{\beta} \sum_{\omega_n} \int d\epsilon \frac{d\rho_{\text{tr}}(\epsilon)}{d\epsilon} G(\epsilon, i\omega_n) e^{i\omega_n 0^+} = \frac{2}{\beta} \sum_{\omega_n} \int d\epsilon \rho_{\text{tr}}(\epsilon) \frac{dG(\epsilon, i\omega_n)}{d\epsilon} e^{i\omega_n 0^+} \end{aligned} \quad (\text{S44})$$

From Dyson's equation,

$$\frac{\partial G(\epsilon, i\omega_n)}{\partial \epsilon} = G(\epsilon, i\omega_n)^2 - F^\dagger(\epsilon, i\omega_n) F(\epsilon, i\omega_n), \quad (\text{S45})$$

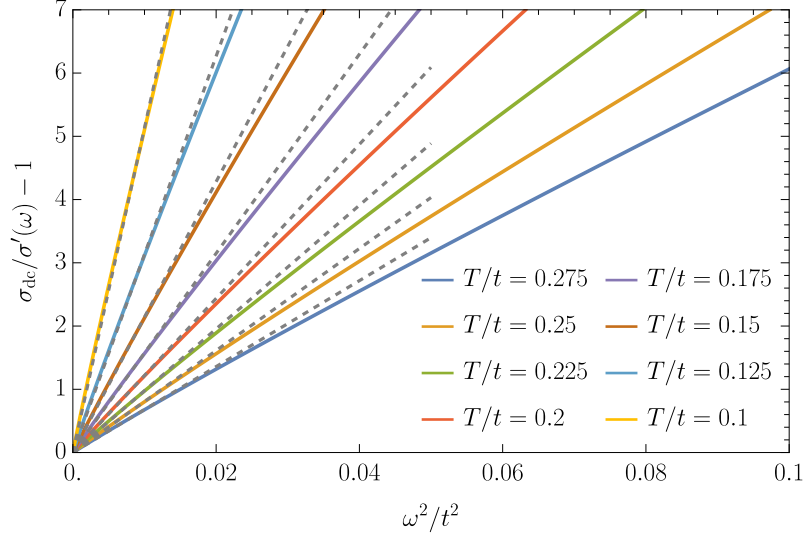

FIG. S10: Linear fits of  $\sigma_{dc}/\sigma'(\omega) - 1$  vs  $\omega^2$  for different temperatures. The gray, dashed lines corresponding to linear fits.

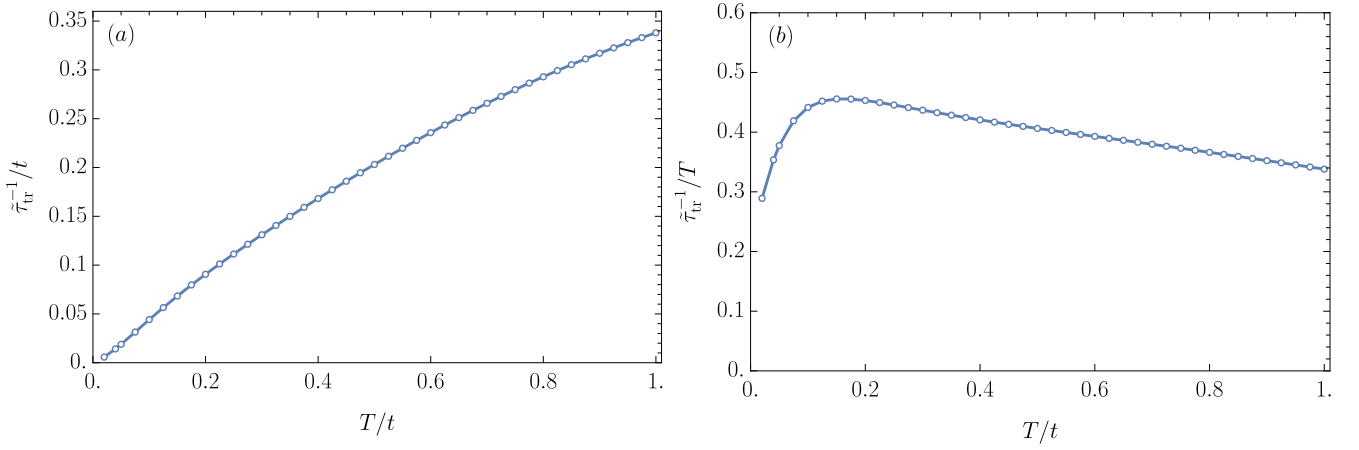

FIG. S11: (a) Transport scattering rate  $1/\tilde{\tau}_{tr}$  extracted from linear fits of  $\sigma_{dc}/\sigma'(\omega) - 1$ . (b) A scaling plot with  $1/\tilde{\tau}_{tr}$  scaled by  $T$ .

and we get for the superfluid stiffness

$$\begin{aligned}
\frac{\rho_s}{\pi e^2} &= \langle -K/2 \rangle - \Lambda(0) \\
&= -T \sum_n \int d\epsilon \rho_{\text{tr}}(\epsilon) (G(\epsilon, i\omega_n)^2 - F^\dagger(\epsilon, i\omega_n) F(\epsilon, i\omega_n)) \\
&\quad + T \sum_n \int d\epsilon \rho_{\text{tr}}(\epsilon) (G(\epsilon, i\omega_n)^2 + F^\dagger(\epsilon, i\omega_n) F(\epsilon, i\omega_n)) \\
&= 2T \sum_n \int d\epsilon \rho_{\text{tr}}(\epsilon) F^\dagger(\epsilon, i\omega_n) F(\epsilon, i\omega_n).
\end{aligned} \tag{S46}$$

## SV. HOMES' LAW

Here we describe the relation between Homes law [8] and our data. To begin, we convert the results of Homes *et al.* [8] to dimensionless units. We use S.I. units throughout for fundamental constants.

Let  $\Sigma$  be the value of the conductivity in  $\text{Ohm}^{-1} \text{ cm}^{-1}$ . Then the conductivity,  $\sigma$ , is

$$\sigma = 100\Sigma \text{ Ohm}^{-1} \text{ meter}^{-1} \tag{S47}$$

Let  $R$  be the value of the superfluid density in  $\text{cm}^{-2}$ , as quoted in Ref. [8]. Then the associated plasma frequency  $\omega_p$  is

$$\omega_p^2 = (100 \times 2\pi c)^2 R \text{ sec}^{-2} \tag{S48}$$

This is connected to our definition of the superfluid density,  $\rho_s$ :

$$\begin{aligned}
\sigma(\omega) &= i \frac{\rho_s}{\hbar \omega} \\
\varepsilon(\omega) &= \varepsilon_0 + \frac{i\sigma(\omega)}{\omega} = -\varepsilon_0 \frac{\omega_p^2}{\omega^2} \text{ as } \omega \rightarrow 0 \\
\Rightarrow \rho_s &= \hbar \varepsilon_0 \omega_p^2
\end{aligned} \tag{S49}$$

So for the dimensionless ratio expressing Homes' Law, we have

$$\begin{aligned}
\frac{\rho_s}{\sigma k_B T_c} &= \frac{\hbar \varepsilon_0 (200\pi c)^2}{100 k_B} \frac{R}{\Sigma T_c} \\
&= 0.024 \frac{R}{\Sigma T_c} \\
&\simeq 2.88,
\end{aligned} \tag{S50}$$

where in the last line we used the value  $R/(\Sigma T_c) \simeq 120$  obtained in Ref. [8].

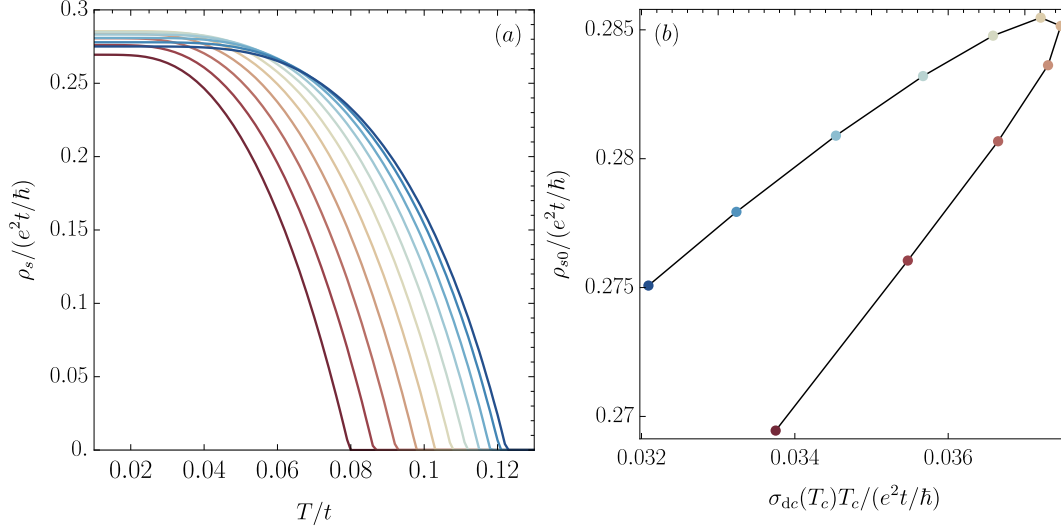

FIG. S12: (a). Temperature dependence of superfluid stiffness  $\rho_s$  at  $g' = 5t^{3/2}$ ,  $v = 0.6$  for various values of renormalized boson mass  $M$ . (b). The plot of zero temperature superfluid density  $\rho_{s0}$  vs  $\sigma_{dc}T_c$  in the unit of  $e^2t/\hbar$ ; the best fit value of the slope for the 5 points closest to the QCP is 2.17.

We show a plot of the superfluid density  $\rho_s$  as a function of  $T$  for various values of distance from the QCP in Figs. 5 and S12. When  $v = 0$ , we find a decreasing  $T_c$  is accompanied by an increasing  $\rho_{s0}$ , the superfluid stiffness at  $T = 0$ , as in Fig. 5. On the other hand, when  $v$  is non-zero, we find that with decreasing  $T_c$ , the stiffness initially increases, and then decreases, as shown in Fig. S12a. For  $v = 0.75$ , the ratio  $\rho_{s0}/(\sigma_{dc}(T_c)T_c)$  takes a value close to (S50), as shown in Fig. S12b.

- 
- [1] D. Hauck, M. J. Klug, I. Esterlis, and J. Schmalian, *Eliashberg equations for an electron-phonon version of the Sachdev-Ye-Kitaev model: Pair breaking in non-Fermi liquid superconductors*, [Annals of Physics](#) **417**, 168120 (2020).
  - [2] I. Esterlis, H. Guo, A. A. Patel, and S. Sachdev, *Large N theory of critical Fermi surfaces*, [Phys. Rev. B](#) **103**, 235129 (2021), [arXiv:2103.08615 \[cond-mat.str-el\]](#).
  - [3] I. Esterlis and J. Schmalian, *Cooper pairing of incoherent electrons: an electron-phonon version of the Sachdev-Ye-Kitaev model*, [Phys. Rev. B](#) **100**, 115132 (2019), [arXiv:1906.04747 \[cond-mat.str-el\]](#).
  - [4] P. M. Dee, K. Nakatsukasa, Y. Wang, and S. Johnston, *Temperature-filling phase diagram of the two-dimensional Holstein model in the thermodynamic limit by self-consistent Migdal approximation*, [Phys. Rev. B](#) **99**, 024514 (2019).
  - [5] J. Schmalian, M. Langer, S. Grabowski, and K. Bennemann, *Self-consistent summation of many-*

- particle diagrams on the real frequency axis and its application to the flex approximation*, Computer physics communications **93**, 141 (1996).
- [6] B. Michon, C. Berthod, C. W. Rischau, A. Ataei, L. Chen, S. Komiya, S. Ono, L. Taillefer, D. van der Marel, and A. Georges, *Reconciling scaling of the optical conductivity of cuprate superconductors with Planckian resistivity and specific heat*, [Nature Communications](#) **14**, 3033 (2023), [arXiv:2205.04030 \[cond-mat.str-el\]](#).
- [7] D. J. Scalapino, S. R. White, and S. Zhang, *Insulator, metal, or superconductor: The criteria*, [Phys. Rev. B](#) **47**, 7995 (1993).
- [8] C. C. Homes, S. V. Dordevic, M. Strongin, D. A. Bonn, R. Liang, W. N. Hardy, S. Komiya, Y. Ando, G. Yu, N. Kaneko, X. Zhao, M. Greven, D. N. Basov, and T. Timusk, *A universal scaling relation in high-temperature superconductors*, [Nature \(London\)](#) **430**, 539 (2004), [arXiv:cond-mat/0404216 \[cond-mat.supr-con\]](#).
